# Supplementary material for: Understanding Radiative Transitions and Relaxation Pathways in Plexcitons
Source: arXiv:2002.05642 ancillary file (2021-03-29)
Supplement: Supplementary file 1 [file supplemental_experimental_procedures.pdf]

# Supplemental Information

## Contents

**1 Details of the linear response fit** **2**

**2 2DES of J-aggregates** **4**

**3 2DES of plasmons** **5**

3.1 A brief overview of relaxation mechanisms in metals . . . . . 5

3.2 2DES spectra of plasmons . . . . . 6

3.3 Kinetics and time constants . . . . . 9

**4 2DES of Plexcitons** **14**

4.1 Early time kinetics . . . . . 16

**5 Details of the simulations of the plexciton 2D spectra** **20**

5.1 Early times simulation . . . . . 23

5.2 Late times simulation . . . . . 27

**6 Supplemental references** **30**

# Note S1. Details of the linear response fit

The fits to the linear absorption of J-aggregates and plasmons are shown in Figures S1 and S2.

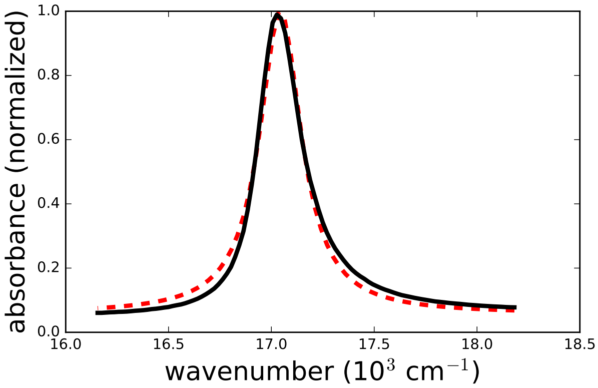


Figure S1: UV-vis absorption of J-aggregates (black solid line) and a Lorentzian fit (dashed red line). Parameters of the fit are reported in Table I of the main text.

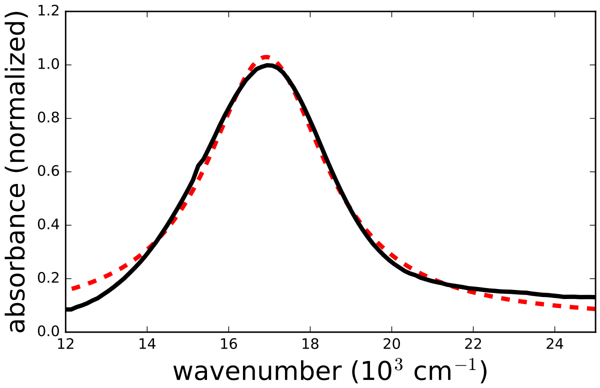


Figure S2: UV-vis absorption of plasmons (black solid line) and a Lorentzian fit (dashed red line). Parameters of the fit are reported in Table I of the main text.

**Global vs. local approach.** The names of the models (local vs. global) refer to the approximations implemented to reach the underlying Markovian master equation [4]. In the global approach, the bath modes couple to the eigenstates of the system, while in the local approach, the bath modes couple to the individual transitions (i.e. the plasmon transition or the J-aggregate bright state). Thus, the two approaches differ in the step at which the interaction with the bath and therefore the dephasing is added. In the global approach, the dephasing rates ($\gamma_a^{(g)}$) are added in the optical response function phenomenologically for each branch, after their energies have been calculated by diagonalizing the Hamiltonian. In the local approach, the dephasing rates for each branch ($\gamma_a^{(l)} \equiv \mathrm{Im}(\omega_a^{(l)})$) correspond to the imaginary part of the energies of each polariton branch, which are obtained by diagonalizing the non-Hermitian Hamiltonian containing dephasing of the plasmon and J-aggregate excited states. Incidentally, it is only the latter approach that generates a characteristic interference-like feature in the absorption spectrum and which allows for a splitting to be observed even though the Rabi frequency is smaller than the dephasing rates.

# Note S2. 2DES of J-aggregates

Fifteen representative 2D spectra are shown in Figure S3. The spectral shape and dynamics are typical for a J-aggregate. The scattering of the excitation pulses is evident in the long-time spectra (>2 ps) and is due to the long tubular structures formed by the TDBC molecules. The fit of the J-aggregates signal at the point of the 2D spectrum marked by the blue dot in Figure 2 of the main text is shown in Figure S4.

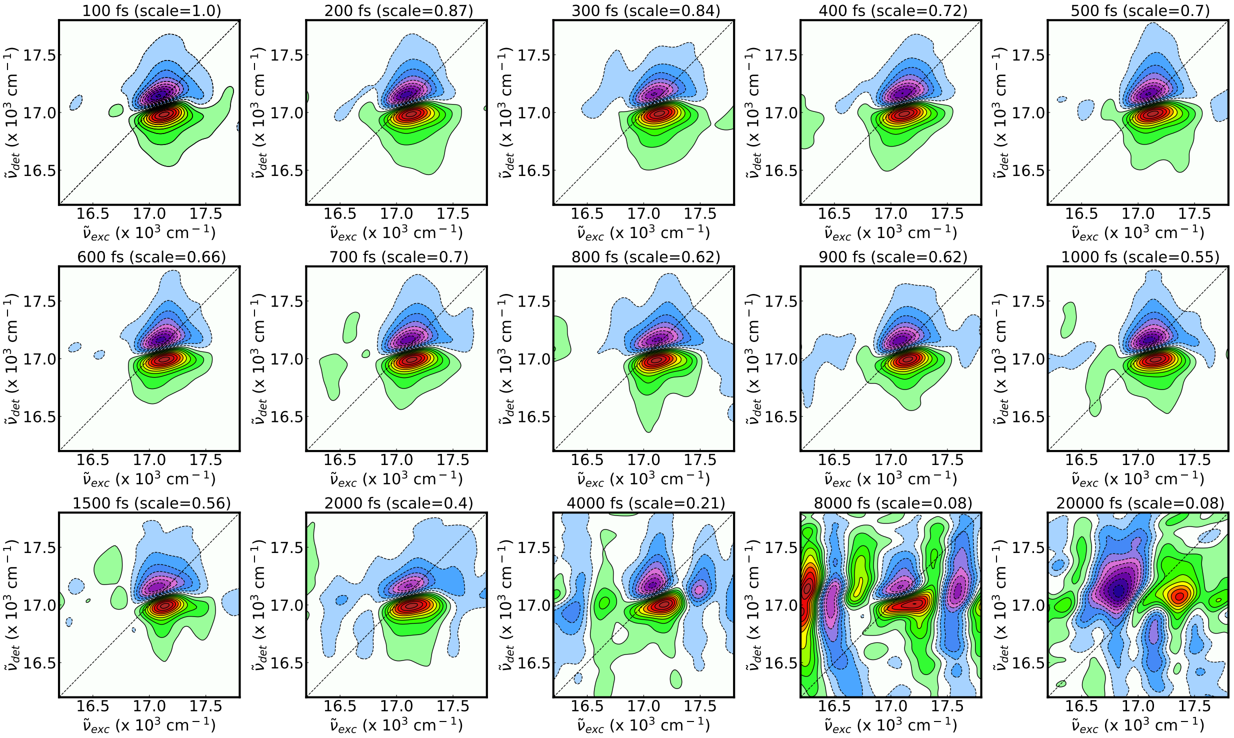


Figure S3: 2D spectra of J-aggregates for representative population times.

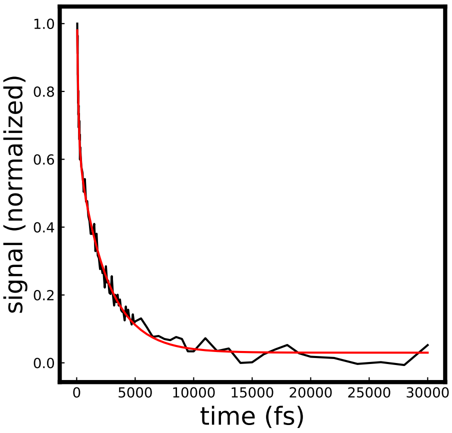


Figure S4: Decay of the J-aggregate signal at the point of the 2D spectrum marked by the blue dot in Figure 2 of the main text, and its fit to a sum of exponentials.

# Note S3. 2DES of plasmons

## S3.1. A brief overview of relaxation mechanisms in metals

We start by briefly describing the expected dynamics for plasmon excitations [10]. The photoexcited plasmon is dephased by Landau or radiation damping in sub-10 fs, and leaves behind a non-equilibrium distribution of hot electron-hole pairs [6, 12]. There are then two main processes which bring the electron distribution back to its equilibrium Fermi distribution: electron-electron (e-e) and electron-phonon (e-ph) scattering. Under the assumption of separation of timescales (i.e. the two-temperature model), the e-e scattering thermalizes the electron distribution before any appreciable energy is lost to the lattice, defining thus an electron temperature. Then the e-ph scattering equilibrates the electron and lattice temperature, thereby raising the temperature of the nanoparticle.

If the deposited thermal energy is high enough, an acoustic mode, often a breathing mode, can be excited resulting in non-trivial ground-state dynamics signals [8]. There are two mechanisms that can excite this mode: 1) the pressure exerted by excited electrons induces a $\delta$-function like force that expands the lattice, and lasts on the order of $\tau_{e-ph}$, and 2) the thermal expansion of the hot lattice, which creates a Heaviside function-like excitation that lasts on the order of $\tau_{\mathrm{phph}}$. The first mechanism does not require any energy to be dissipated inside the nanoparticle while the second one does.

The excited eigenmode results in an oscillation of the third-order (i.e. pump-probe) signal that can be fit by the

cosine function $S \propto \cos(\omega_0 t - \phi)$ (see equation (4) of the main text or equations (S.1) and (S.2) of the supporting information). $\phi$ is often referred to as the asymptotic phase and each of the mechanisms described result in a different value of the asymptotic phase [11], shifted by $90^o$. The phase for the hot electron pressure (also called deformation potential) is $\pi/2 + \arctan(\omega_0 \tau_{e-ph})$ (resulting in a sine-like oscillation for typical $\omega_0$ and $\tau_{e-ph}$ values in metals) while the phase for the hot (displacive) lattice mechanism is $\phi \approx \arctan(\omega_0 \tau_{e-ph})$ (resulting in a cosine-like oscillation).

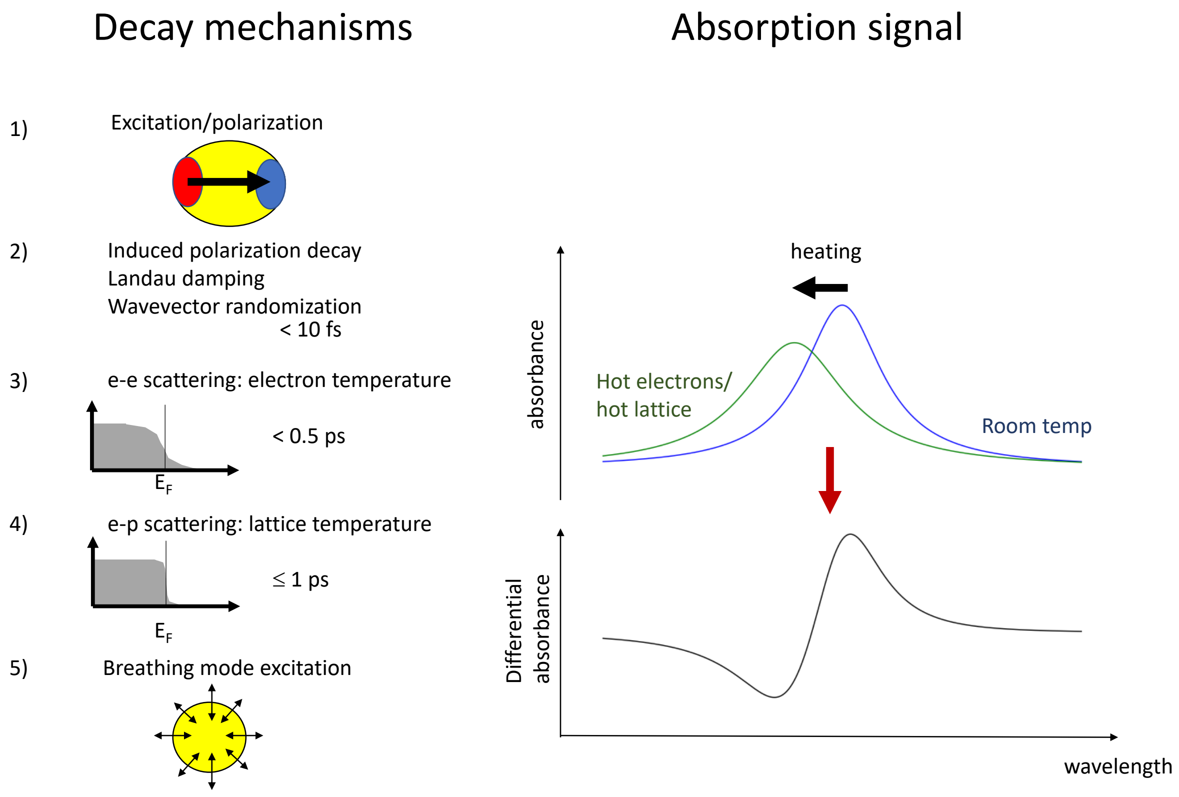


Figure S5: Dissipative processes in plasmonic nanoparticles. Left: plasmon decay mechanisms along with their respective typical timescales. Right: absorption spectrum of a hot and cold plasmon, along with the differential absorption that characterizes the pump-probe spectrum at long times (>4 ps). During the time period when the acoustic eigenmode is present, the volume of the lattice oscillates changing the resonance frequency of the plasmon transition, which produces an oscillatory signal in the differential absorption.

## S3.2. 2DES spectra of plasmons

Fifteen representative 2D spectra for Ag nanoprisms are shown in Figure S6 (top). The dynamics show a dispersive signal with bandshift occurring below 2 ps and a sign reversal of the signal for times beyond 4 ps. In Figure S6

(bottom) pump-probe spectra are shown of the same nanoparticles with a zoomed-in scale of the region probed by the 2D spectrum.

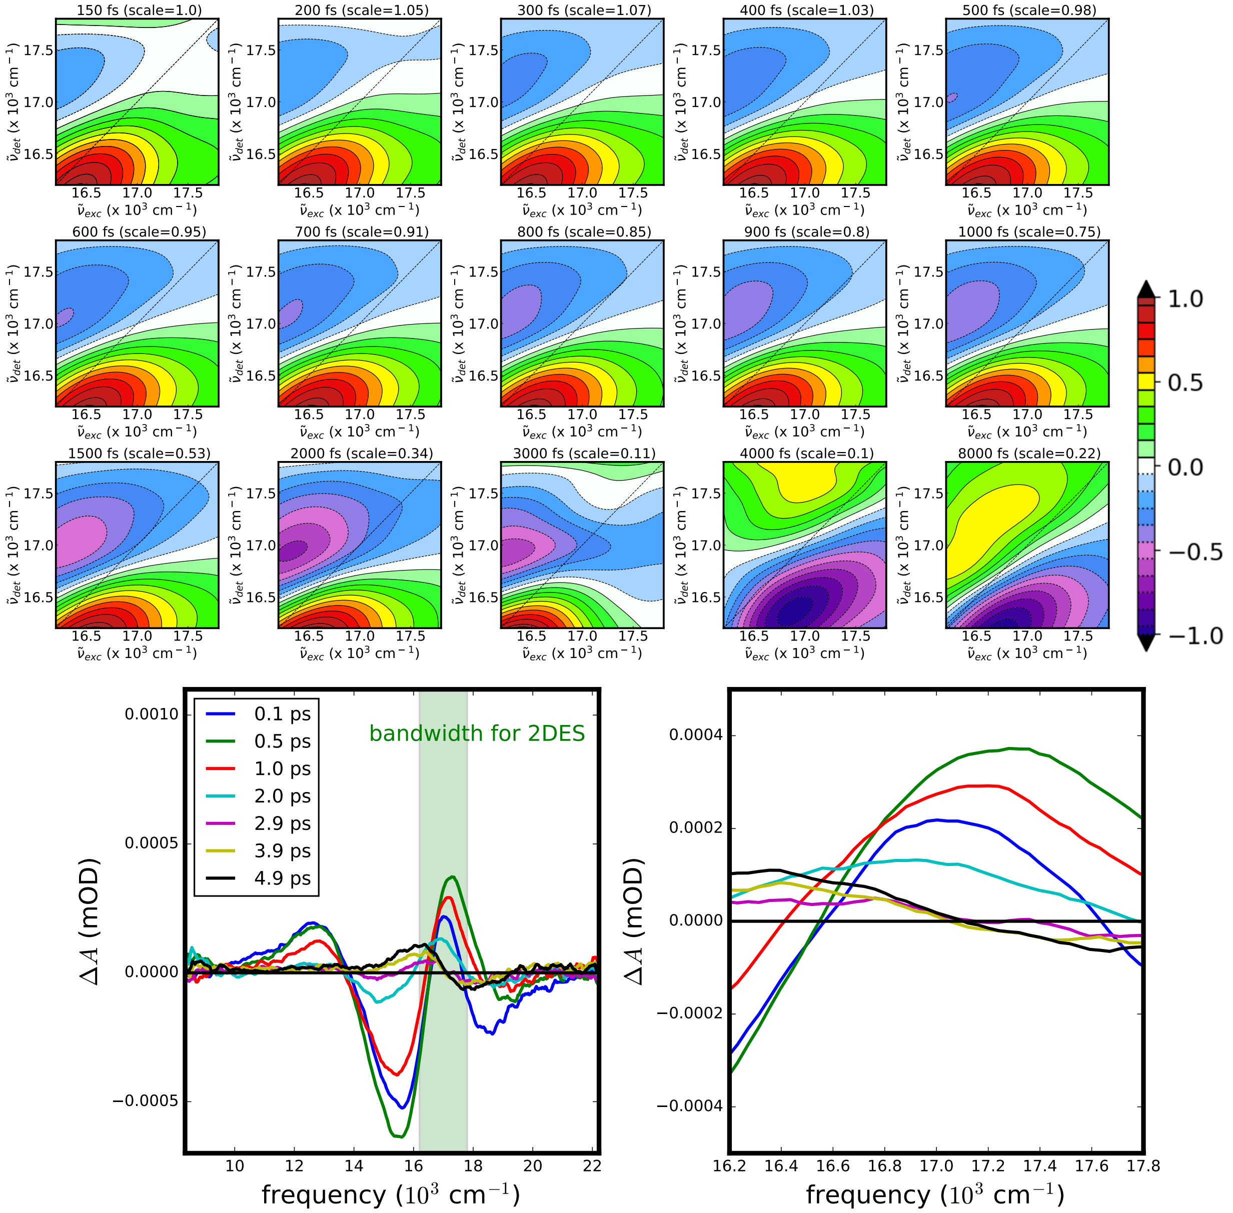


Figure S6: 2DES and transient absorption of plasmonic nanoparticles. Top: 2D spectra of Ag nanoparticles for representative population times. Bottom: Pump-probe spectra of the same Ag plasmons. The pump-probe data is taken at 1 kHz repetition rate using 50-fs, 6 nJ pulses centered at 590 nm (left). The data have been smoothed with a Savitsky-Golay algorithm with a window size of 330 cm$^{-1}$ and a polynomial order of 3. The right graph shows a close-up of the region probed by the 2DES measurements (green region in the full scale spectrum). The pump-probe spectrum shows differential absorption (pump on - pump off) where the GSB and SE show up as negative features and ESA as a positive feature, in contrast to the 2D spectra where GSB and SE are positive, while ESA appears as negative.

## S3.3. Kinetics and time constants

We now use the kinetic traces from the pump-probe and the 2D maps to extract the parameters of Equation 4 of the main text, reproduced below:

$$\begin{aligned} I(t) &= A_1(1 - e^{-t/\tau_{ee}})e^{-t/\tau_{eph}} \\ &+ A_2(1 - e^{-t/\tau_{eph}})e^{-t/\tau_{phph}} \\ &+ A_3(1 - e^{-t/\tau_{eph}})e^{-t/\tau_{vib}} \cos(\omega_0 t - \phi) \\ &+ A_4(1 - e^{-t/\tau_{eph}})e^{-t/\tau_{vib}} \end{aligned} \tag{S.1}$$

where $\tau_{ee}$ and $\tau_{eph}$ are the e-e and e-ph scattering times, $\omega_0$ is the angular frequency of the breathing mode, $\phi$ its phase, and $\tau_{vib}$ ps its dephasing time, $\tau_{phph}$ is the phonon-phonon scattering time. An additional term $A_4(1 - e^{-t/\tau_{eph}})e^{-t/\tau_{vib}}$ has to be added to obtain a good fit compared to the model developed in [9, 5] and can represent anharmonicity of the mode.

We focus first on the long-time dynamics given by the oscillatory signal of the acoustic eigenmode. It is important to know the phase $\phi$, as it helps to distinguish between the excitation mechanism. As mentioned above, a mode excited by hot electron pressure (fast thermal expansion) has an asymptotic phase predicted at $\phi = \arctan(\omega_0\tau_{e-ph}) = 28^o$ ($\phi = \arctan(\omega_0\tau_{e-ph}) + 90^o = 118^o$), where we have used the time constants and angular frequencies extracted from the fits shown in Figure S8.

Figure S7.a shows three representative pump-probe traces. The kinetic trace at each probe frequency is fit by an oscillatory signal and an exponential decay which is a simplified fit of Eq. (S.1) for long times (see a representative kinetic trace and fit in Figure S7.b):

$$S = Ae^{-t/\tau_{vib}} \cos(\omega_0 t - \phi) + Be^{-t/t_{vib}} + C \tag{S.2}$$

Figure S7.c and Figure S7.d shows the fits for the asymptotic phase $\phi$ and the angular frequency $\omega_0$ at each probe frequency. We notice that the acoustic eigenmode frequency is not the same for all probe frequencies, being slightly larger in the region marked in blue in the figure. This can happen either because of the proximity of the nodal line where the oscillation is less prominent, or due to the presence of an additional eigenmode. The relatively

fast dephasing of the acoustic eigenmode makes it difficult to discern a second mode via fitting, so that we exclude the blue region from our averages. Indeed, the phase in the blue region becomes negative indicating that our single eigenmode model does not capture the optical response in that region of the probe frequency. Averaging over the white region, we get a value for the asymptotic phase of $\phi = 25^o$. It is important to note that to distinguish between the two mechanisms we need to ascertain if the phase is closer to $28^o$ or to $118^o$ so that the phase variation present in the fit of the pump-probe data is not critical.

We also fit kinetic traces of representative points of the 2D map using S.1 (see Figure S8 and Figure S9 for early and late times, respectively). We see that the fit works well for the non-equilibrium dynamics as well as the late ground state acoustic eigenmode dynamics. We obtain $\tau_{ee} = 300 \pm 200$ fs and $\tau_{e-ph} = 1.4 \pm 0.2$ ps. From these values we calculate the predicted phase of $\phi = \arctan(\omega_0 \tau_{e-ph}) = 28^o$ for the hot lattice (displacive) mechanism.

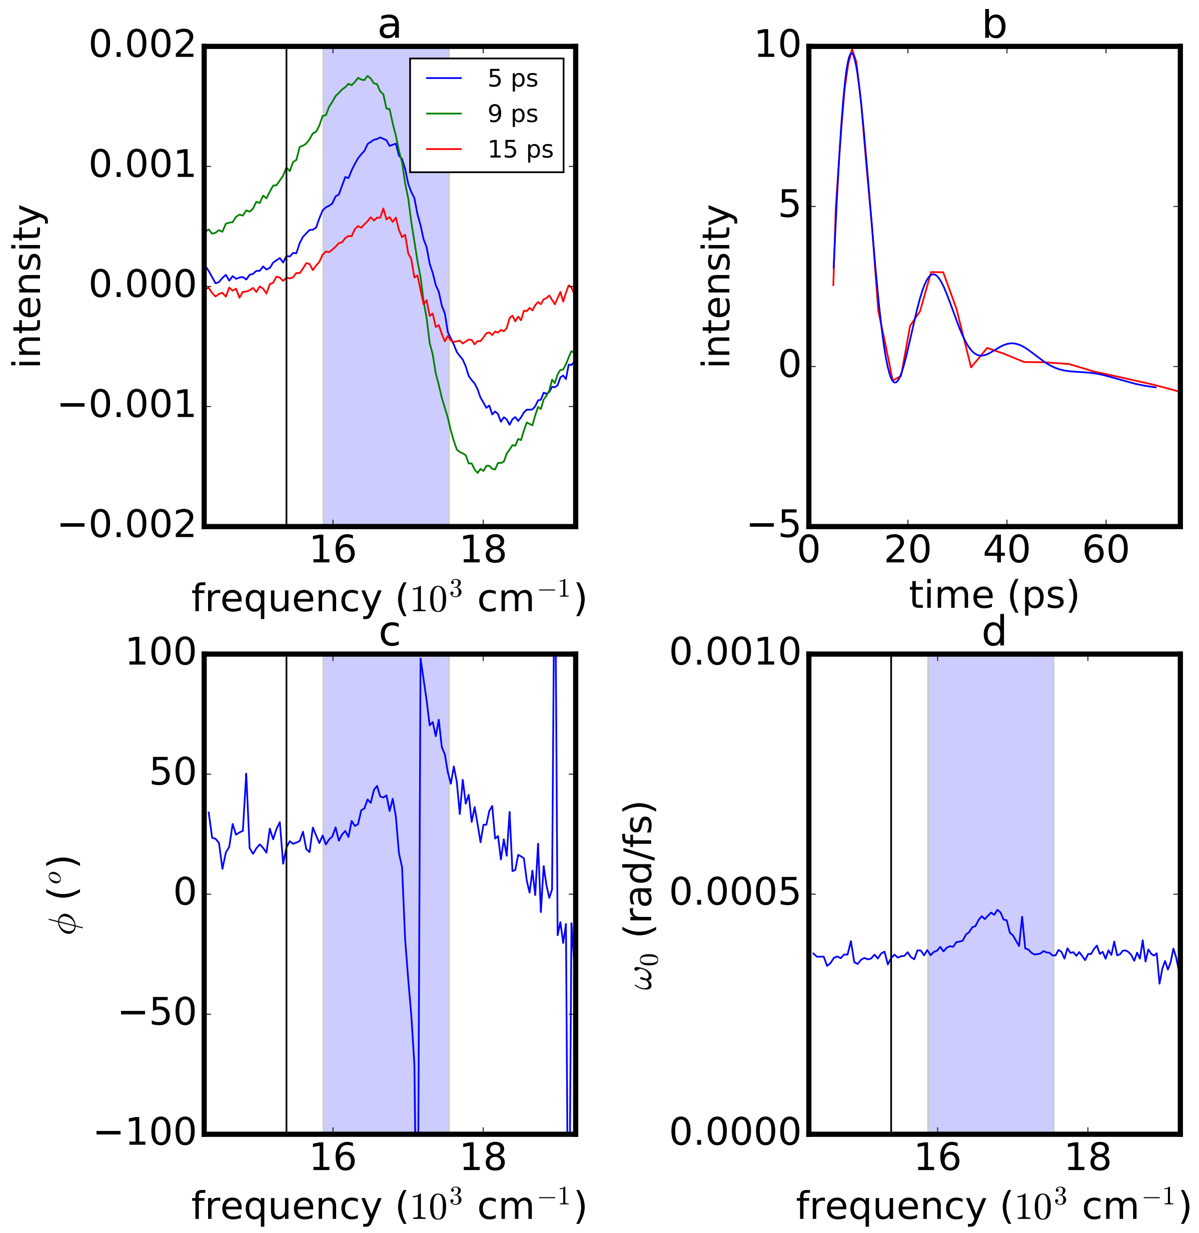


Figure S7: Asymptotic phase of acoustic eigenmodes in plasmonic nanoparticles. a) Transient spectra at three delay times corresponding to ground state dynamics. b) Characteristic time trace at 15,400 cm$^{-1}$ along with a fit of the oscillations. c) Phase of the oscillation as a function of probe frequency. The vertical line marks the position of the time trace shown at b). The shaded blue rectangle marks the frequency range where phases are excluded from the average (see text). d) Angular frequency of the fitted oscillation. The vertical line marks the position of the time trace of b). The shaded blue rectangle marks the frequency range where frequencies are excluded from the average (see text).

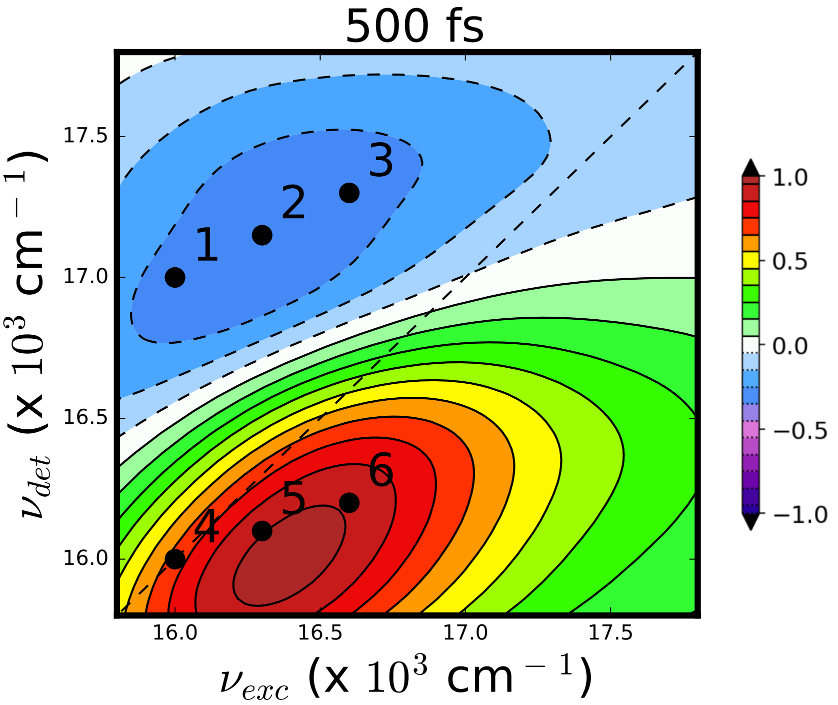


(b)

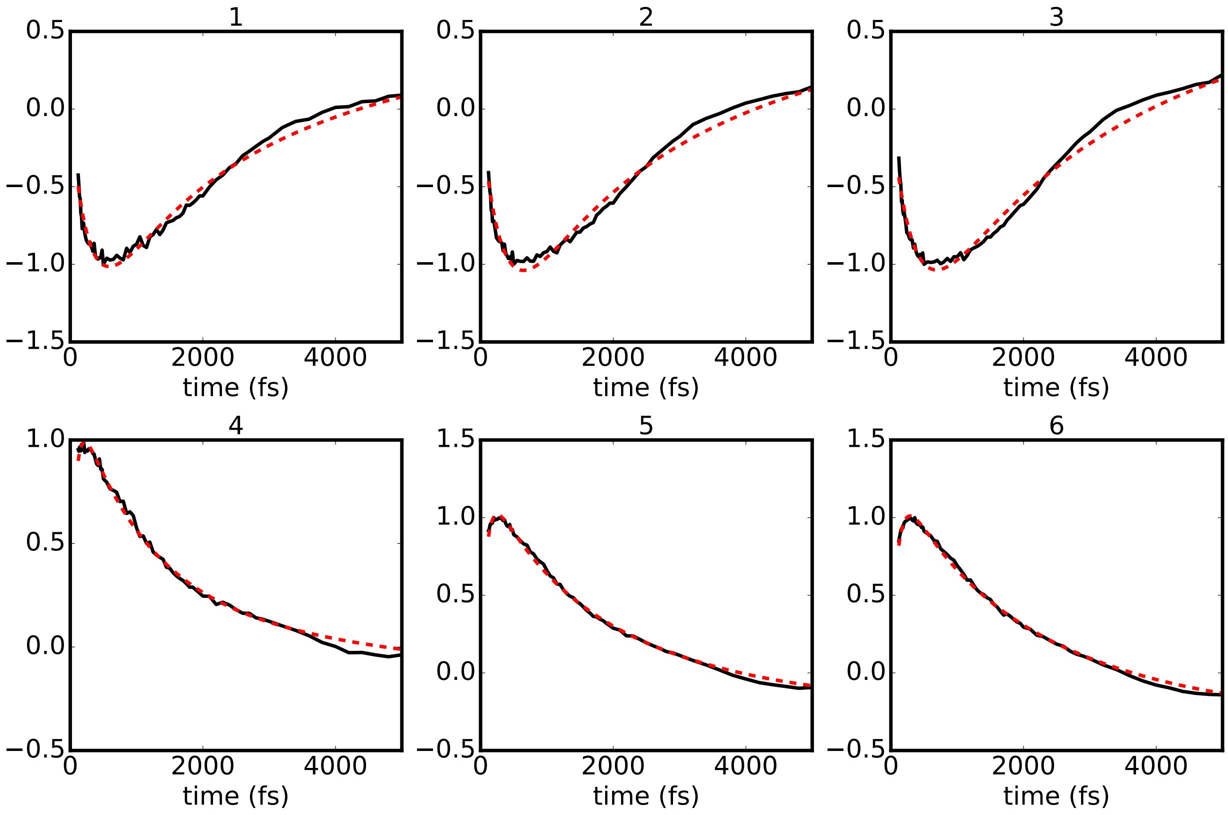


Figure S8: Early time dynamics of excitations in plasmonic nanoparticles. Time traces of indicated points in the 2D spectrum of Ag plasmonic nanoparticles along with the fit resulting from Equation S.1. The graphs show the non-equilibrium electron dynamics at early population times.

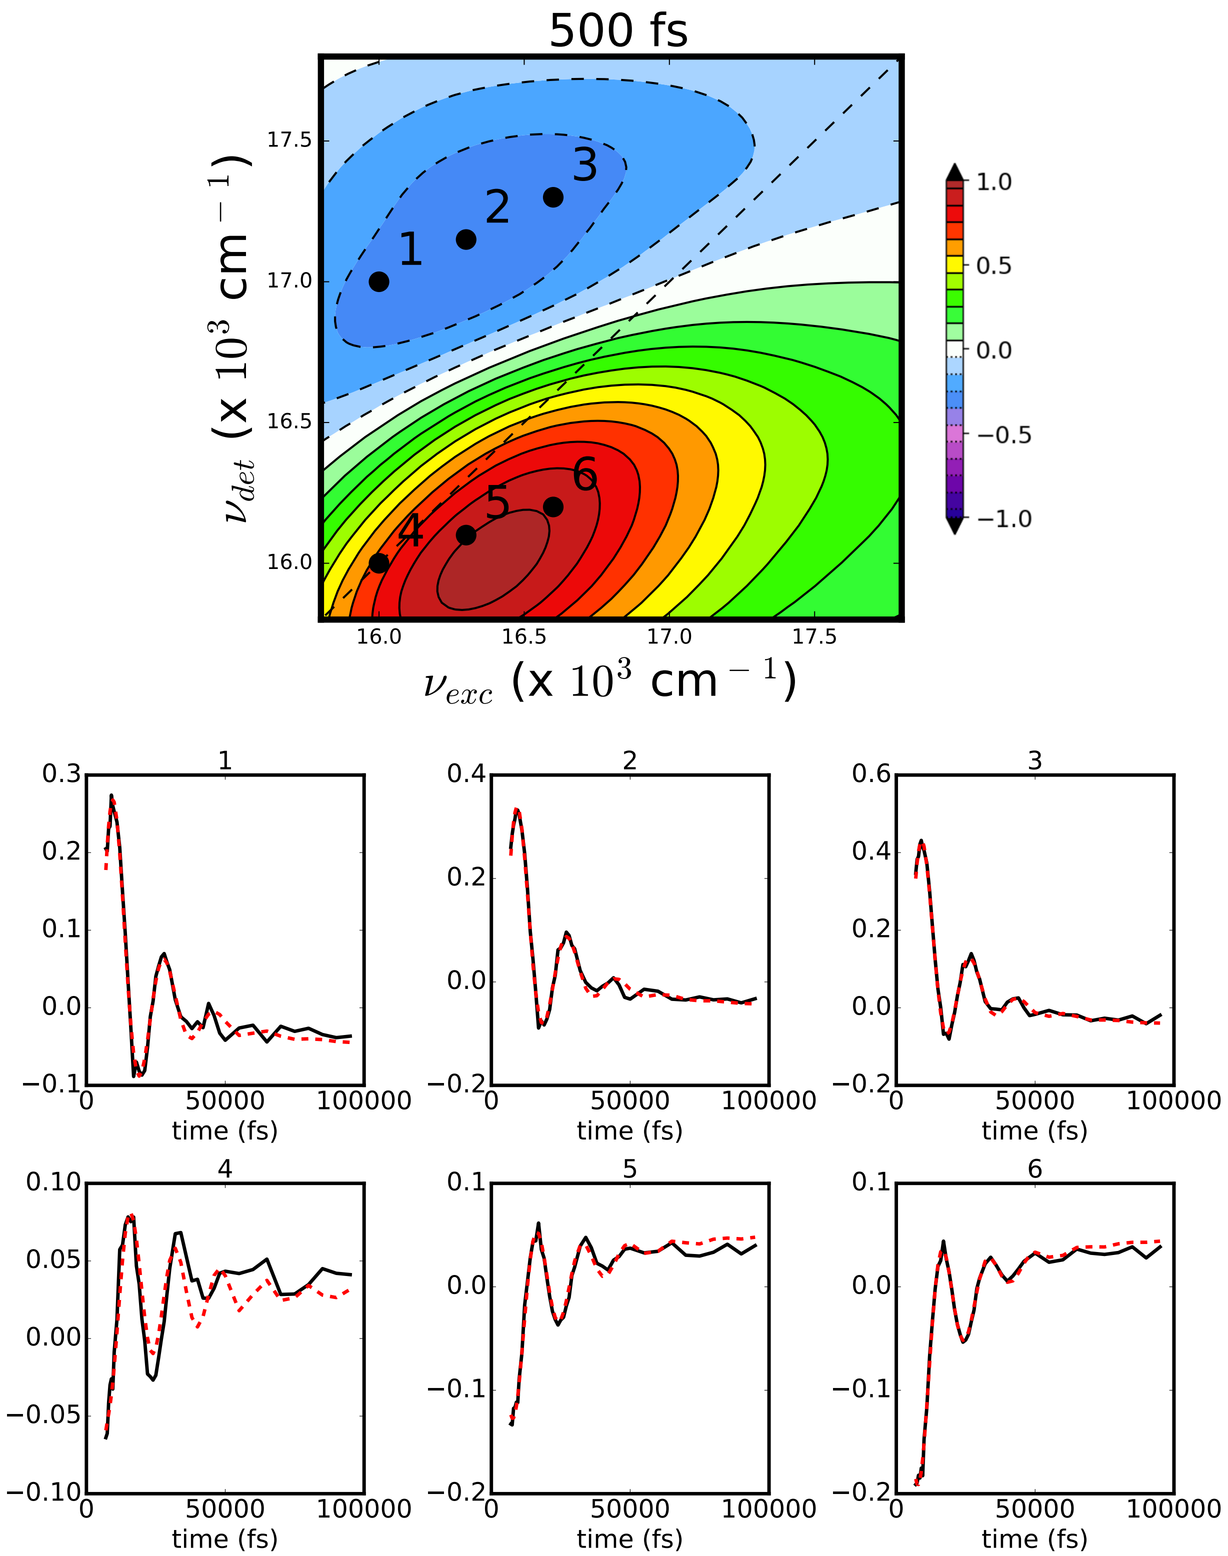


Figure S9: Late time dynamics of excitations in plasmonic nanoparticles. Time traces of indicated points in the 2D spectrum of Ag plasmonic nanoparticles along with the fit resulting from Equation S.1. The graphs show the ground state dynamics at late population times.

# Note S4. 2DES of Plexcitons

Fifteen representative 2D spectra of plexcitons are shown in Figure S10. We can clearly see that the lineshape remains unchanged for the first 700 fs, followed by a spectral shift that can be observed up to 8 ps.

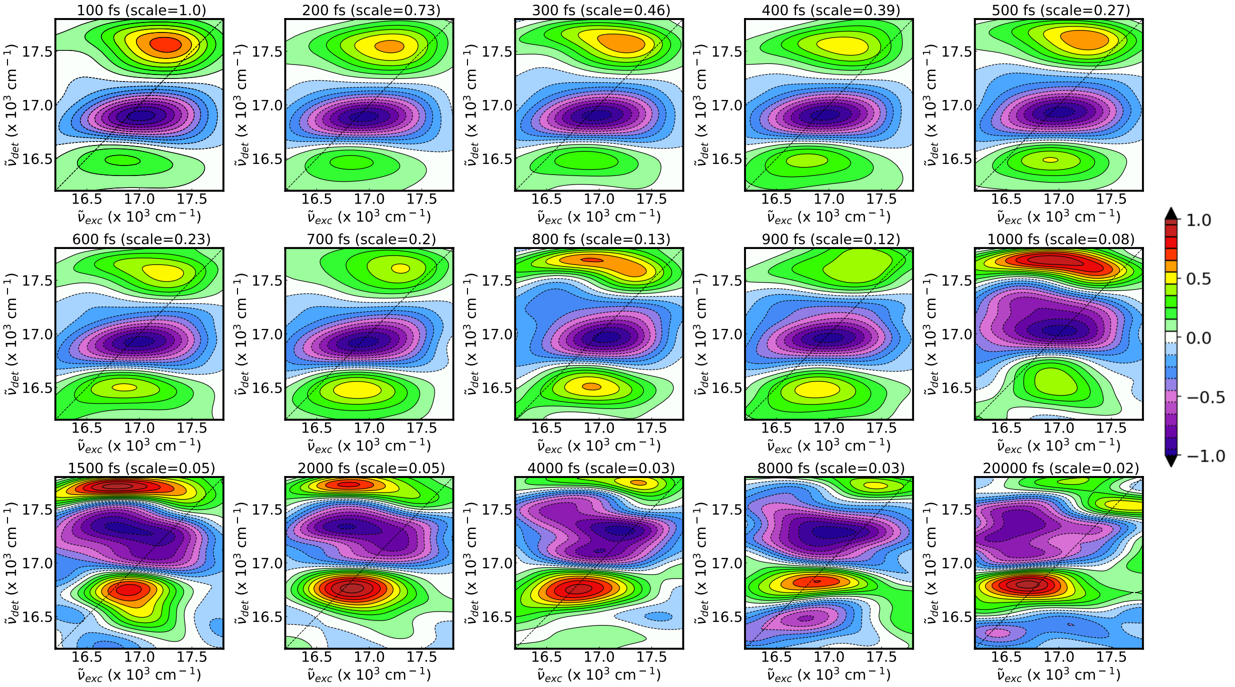


Figure S10: 2D spectra of plexcitons at representative population times.

The dynamics are well described by a global fit of 4 exponential time constants of $40 \pm 20$ fs, $400 \pm 100$ fs, $1.6 \pm 0.6$ ps and a very long decay contribution that appears constant in the time range studied (see Figure S11 and S12). This long time signal is distinguished from the background noise although its amplitude is only 1% of the total initial signal (See Figure S13). This long-time signal agrees reasonably well with our simulations for a plexciton in a hot ground state plexciton (see Figure 3 of the main text).

Calculated residuals to the fit of the time dynamics consists of a weak oscillatory signal. We Fourier transform the residuals to obtain a frequency spectrum that shows vibrational, electronic or vibronic coherences present in the signal. We observe the high-amplitude modes at 675 cm$^{-1}$ and 1200 cm$^{-1}$ which match very well the Raman modes of TDBC, which are enhanced on the Ag surface (see Figure S14, [1]).

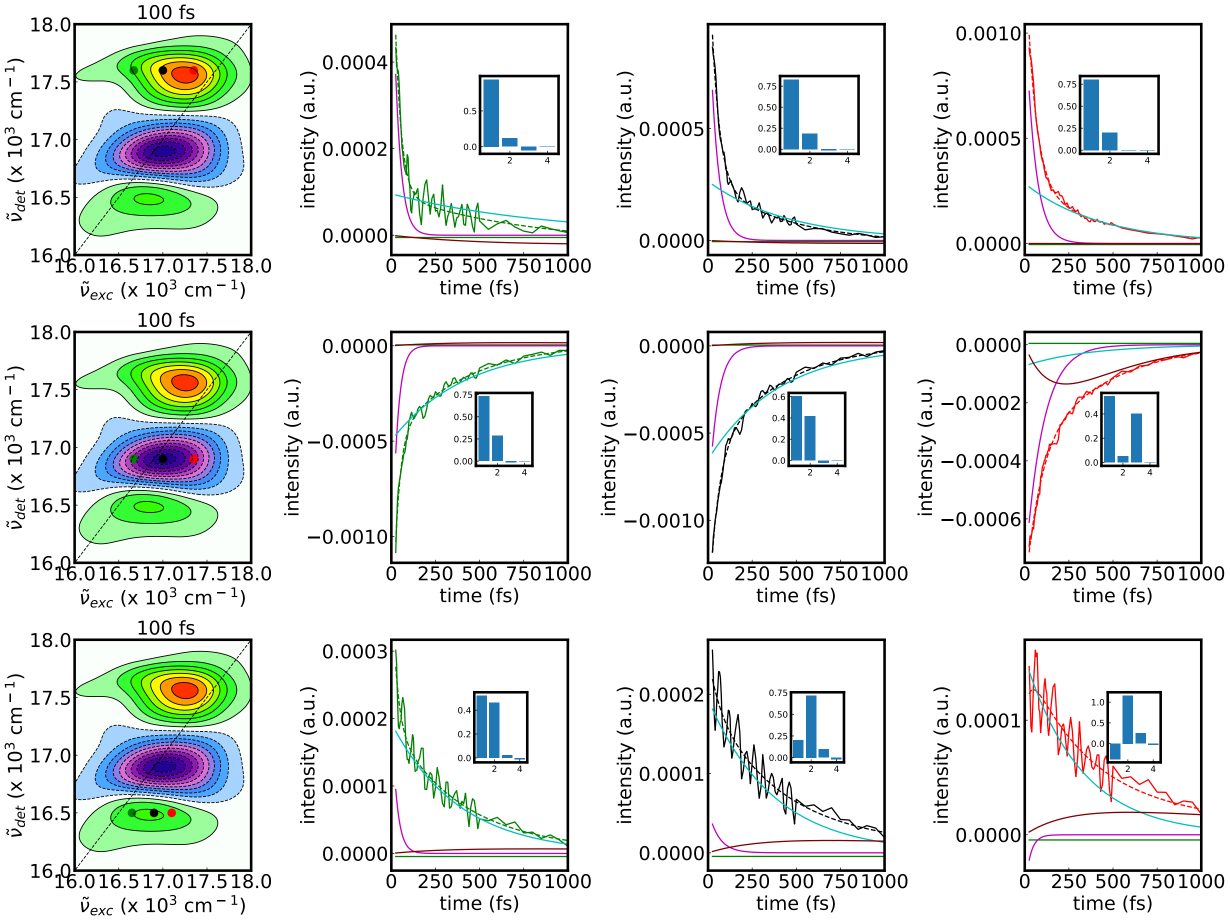

Figure S11: Early time dynamics for selected points in the plexciton 2D spectra. The data, fit and its decomposition into single kinetic traces is shown in the figures to the right of the 2D spectra. The insets show the fractional amplitude associated to each time constant.

## S4.1. Early time kinetics

It is important to discuss in detail the fastest plexciton decay component since it has the largest amplitude of the dynamics. The fast component has been interpreted in the past as a relaxation from the bright molecular state to the dark state manifold present in J-aggregates. Indeed, this is the observation in J-aggregates in solution. However, the amplitude of the fast component (see Figure S11, insets) cannot be ascribed only to the loss of the stimulated emission pathway, but has to correspond to a decrease of the ground-state bleach (i.e. decay of the excitation back to the ground state). Consistent with this observation we attribute this ultrafast component to radiation damping accelerated by the large Purcell factor brought about by the plasmonic nanoparticle. We can however not rule out that the loss of signal does not come from excitation transfer to molecular dark states. Due to the complex nature of the couplings between plasmonic mode and J-aggregates, between the states of the metallic band structure and J-aggregates, coupled to the 20 fs time resolution limitation imposed by the laser pulse duration, it is difficult to unambigously assign this initial time constant.

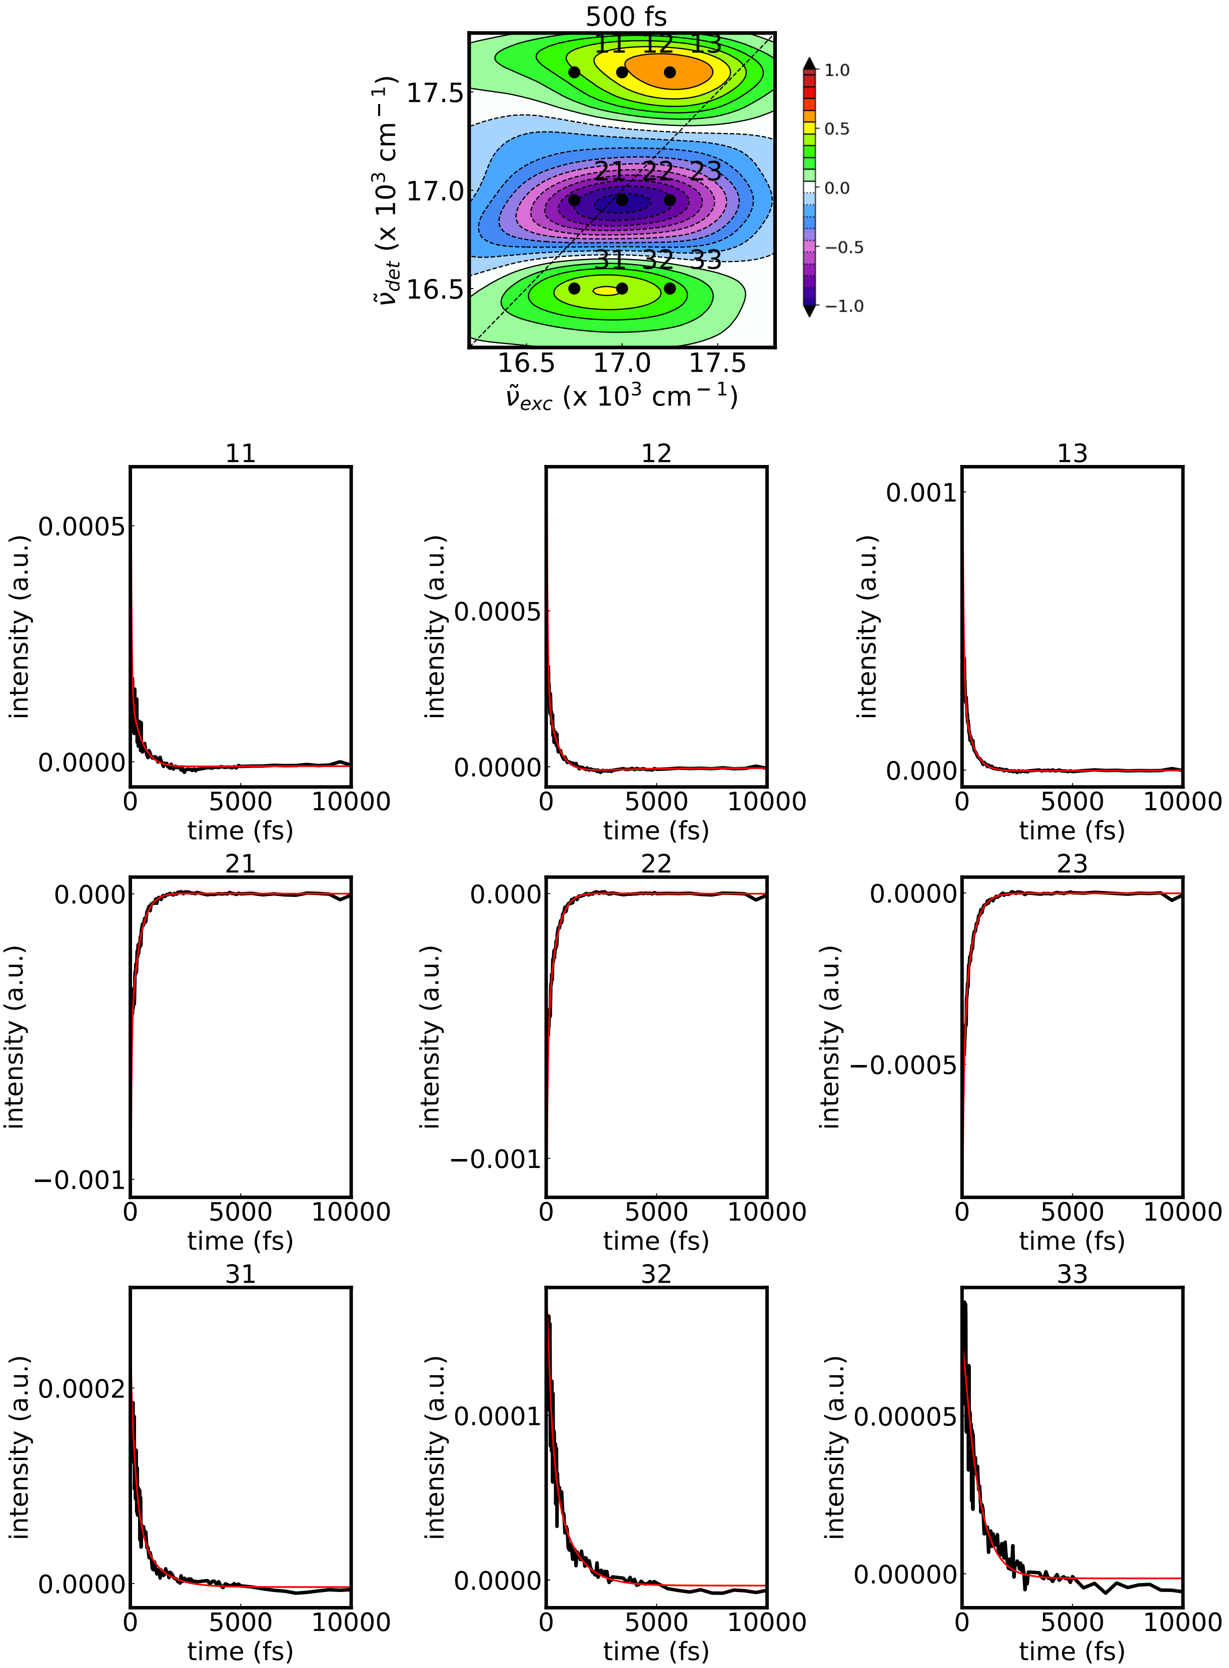




Figure S12: Time traces for plexcitons and fits for a set of representative points shown in the 2D spectra above.

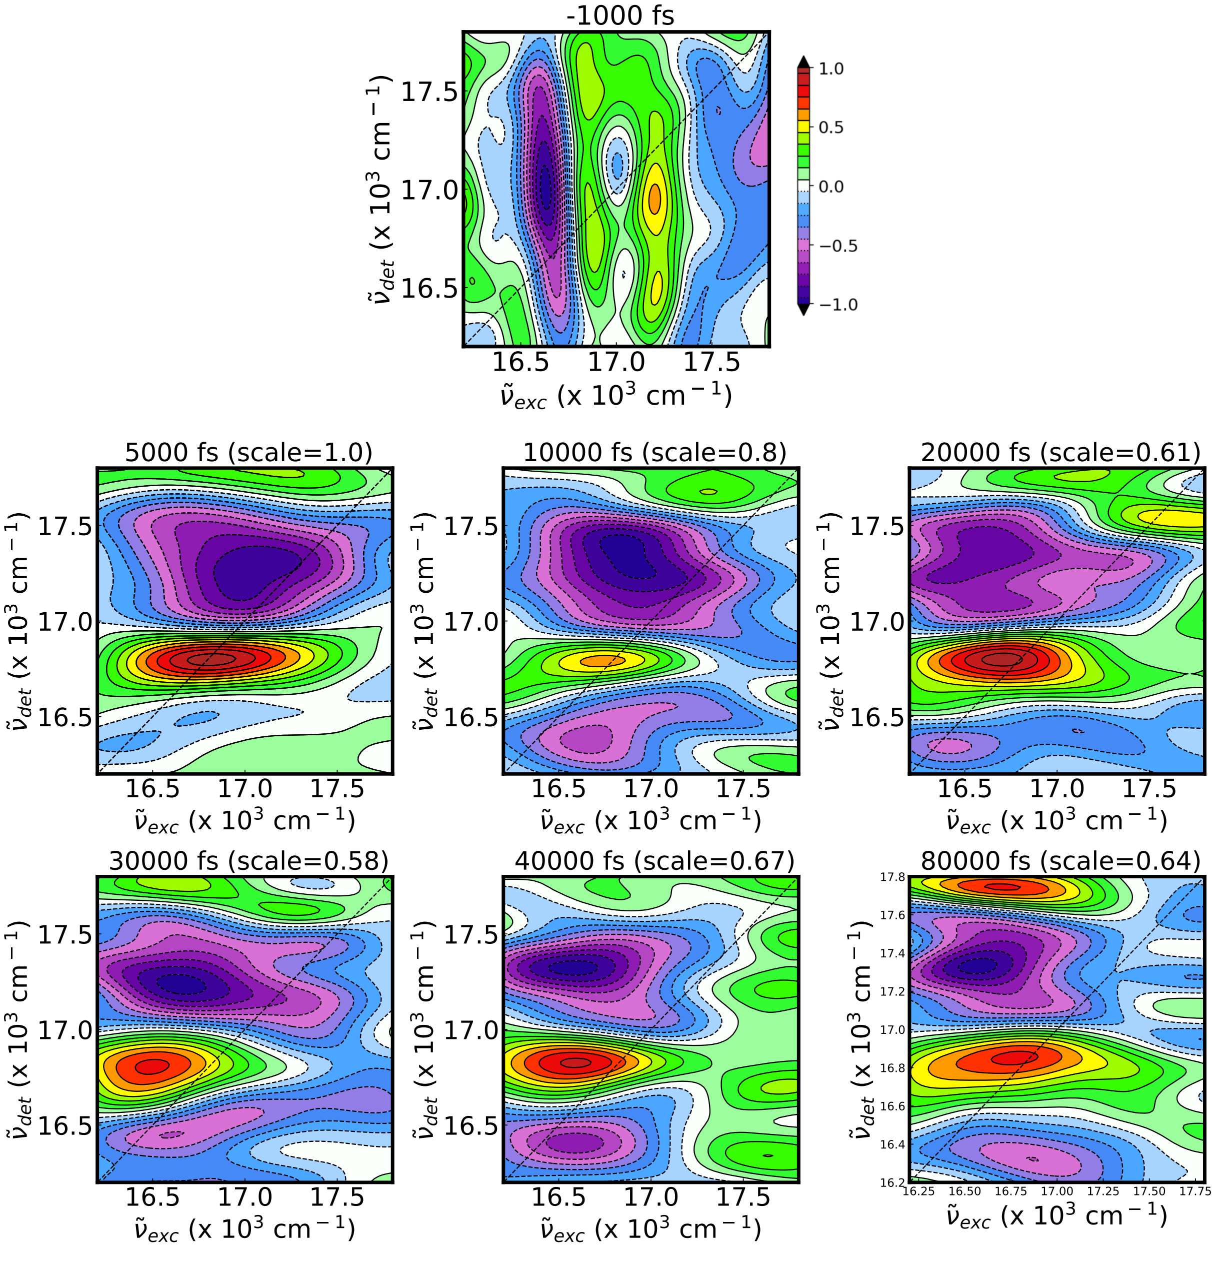


Figure S13: Long time 2D spectra for plexcitons. The long time signal shows a residual signal, which is consistently different from the signal-free background (taken at -1 ps).

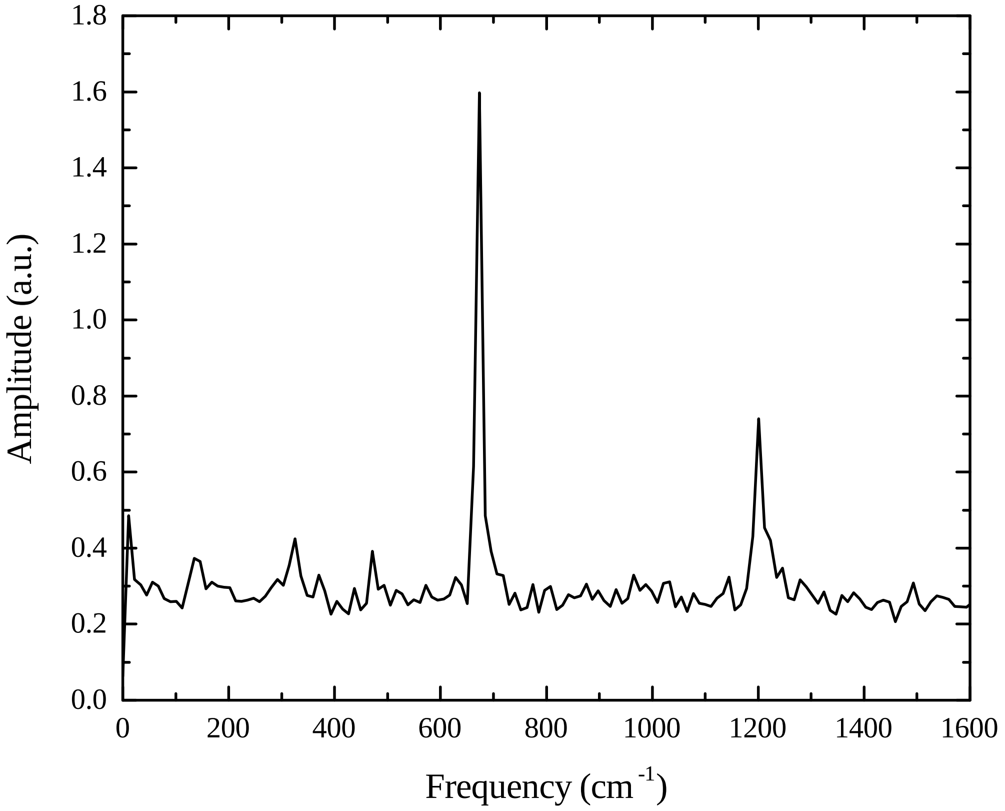


Figure S14: Fourier transform spectrum of the residual to the fit of the kinetic traces (see text). The frequency spectrum reveals any oscillatory components of the signal corresponding to vibrational, electronic or vibronic coherences. For plexcitons, the observed peaks correspond to the vibrations observed in surface-enhanced Raman Spectroscopy of TDBC on Ag nanoparticles ([1]).

## Note S5. Details of the simulations of the plexciton 2D spectra

Here, we provide details of the simulation of the 2D spectra based on the energy structure depicted in Figure 1.a and Table II of the main text. Briefly, we calculate the contributions of the different Feynman diagrams [7] and correct for the finite pulse duration according to Do et al. [2] (see Figure S15 for the pulse spectral profile and its Gaussian fit):

$$\begin{aligned} S(\omega_t, T=0, \omega_\tau) = {} & R_{NR}(\omega_t, \omega_\tau)\mathcal{E}_1(\omega_\tau - \omega_L)\mathcal{E}_2^*(\omega_\tau - \omega_L + i\gamma)\mathcal{E}_3(\omega_t - \omega_L + i\gamma)E_{LO}^*(\omega_t) \\ & + R_R^*(\omega_t, -\omega_\tau)\mathcal{E}_1(\omega_\tau - \omega_L)\mathcal{E}_2^*(\omega_\tau - \omega_L - i\gamma)\mathcal{E}_3^*(\omega_t - \omega_L + i\gamma)E_{LO}(\omega_t) \end{aligned} \tag{S.3}$$

where $R_{NR}$ and $R_R$ are the non-rephasing and rephasing response functions, respectively, and $\mathcal{E}_i$ is the Fourier transform of the $i$–th pulse envelope of center frequency $\omega_L$. $\omega_t$ and $\omega_\tau$ are the detection and excitation frequencies, respectively. The expressions allow for an exponential decay during the pulse duration with rate $\gamma$. The chosen Feynman diagrams (Fig. S16) reflect the physics of the process and vary for early or late times: at early times the nonlinearity arises from a system with $fN$ molecules in the excited state (where $f$ is the excited fraction and $N$ the total number of molecules per nanoparticle), and at late times it arises from a hot ground state that has a different linear response than at room temperature.

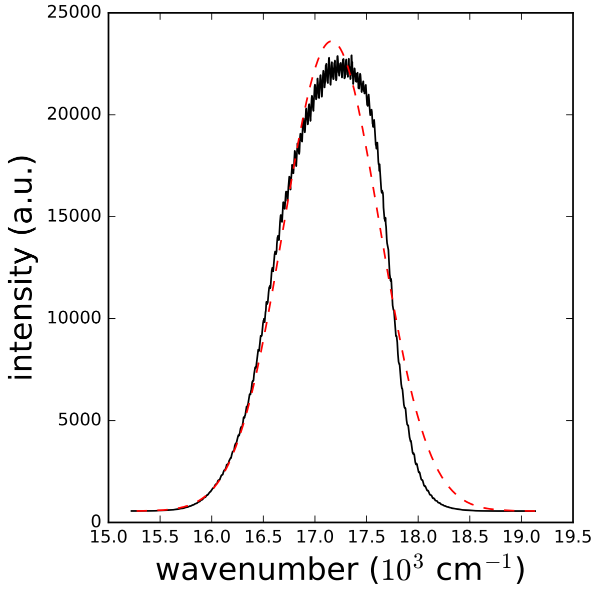


Figure S15: Laser spectrum used in 2DES experiments and its Gaussian fit used for the simulations.

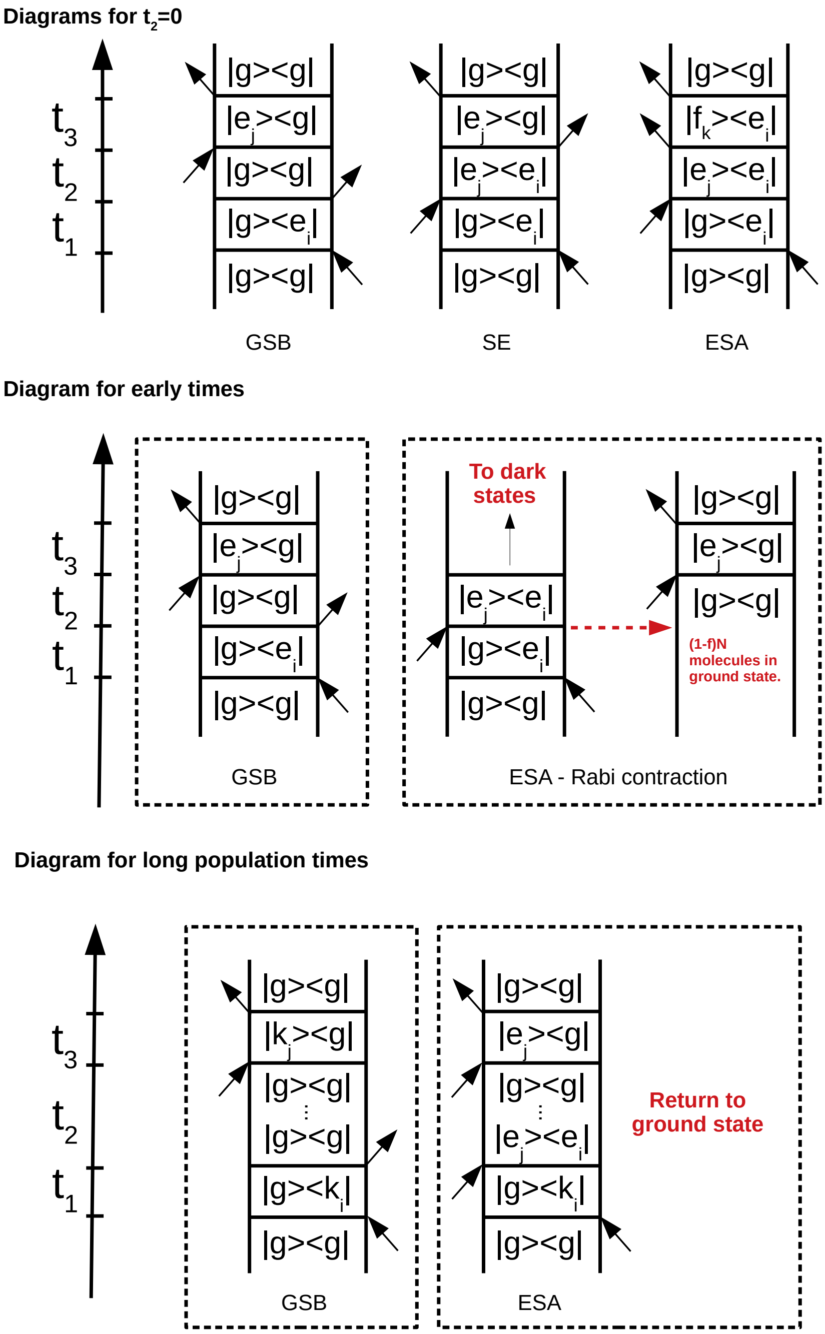


Figure S16: Feynman diagrams. Rephasing Feynman diagrams describing the signal for $t_2 = 0$, for very early times (after plasmon dephasing and injection to molecular dark states has taken place) and for long population times (long enough for the electron distribution to be in thermal equilibrium with the lattice)

## S5.1. Early times simulation

At $t_2 = 0$, the plasmon has not had time to dephase and the signal corresponds to a system comprising only of discrete levels. The Feynman diagrams for such as system generically consist of the top diagrams of Figure S16. However, due to pulse overlap effects we cannot measure exactly at $t_2 = 0$. For slightly longer times, we assume that the SE and ESA contributions that evolve along an excited state during $t_2$ become negligible due to transfer to dark states and dephasing. We thus consider the set of diagrams of Figure S16 (middle row) where the nonlinearity comes from a Rabi contraction [3]. After the initial pair of pulses, a fraction $f$ of the total number of molecules per nanoparticle $N$ have been excited, leaving $(1 - f)N$ molecules in the ground state. When the third pulse arrives, it sees a modified ground state where the vacuum Rabi splitting has contracted by a factor $\sqrt{1 - f}$. In principle other nonlinearities affecting the transition energies (excitation induced shift), dephasings (excitation induced dephasing) and the transition dipole moment strengths are possible.

We show in Figures S17 (local approach) and S18 (global approach) the simulations for early times with finite pulses (full fill) and in the impulsive limit (semi-transparent fill). The number of parameters and the finite bandwidth makes it challenging to obtain a unique fit. We show one family of parameters in Tables S1 and S2 , while an unambiguous fit will have to be postponed until broadband experiments are available.

| Parameters | Ground state | Excited state |
|---|---|---|
| $\tilde{\nu}_{P1}$ ($10^3$ cm$^{-1}$) | 19.21 | 20.17 |
| $\tilde{\nu}_{J1}$ ($10^3$ cm$^{-1}$) | 16.82 | 15.98 |
| V ($10^3$ cm$^{-1}$) | 0.98 | 0.88 |
| $\mu_{p1}$ | 1 | 0.95 |
| $\mu_{j1}$ | 0.048 | 0.043 |
| $\gamma_{P1}$ ($10^3$ cm$^{-1}$) | 3.31 | 3.31 |
| $\gamma_{J1}$ ($10^3$ cm$^{-1}$) | 0.158 | 0.158 |
| $1/\gamma_{P1}$ (fs) | 1.6 | 1.6 |
| $1/\gamma_{J1}$ (fs) | 34 | 34 |

Table S1: Parameters for the early times 2DES simulation in the local approach.

| Parameters | Ground state | Excited state |
|---|---|---|
| $\tilde{\nu}_{P1}$ ($10^3$ cm$^{-1}$) | 19.52 | 20.69 |
| $\tilde{\nu}_{J1}$ ($10^3$ cm$^{-1}$) | 16.08 | 17.21 |
| V ($10^3$ cm$^{-1}$) | 0.98 | 0.88 |
| $\mu_{p1}$ | 1 | 1 |
| $\mu_{j1}$ | 0.05 | 0.045 |
| $\gamma_{UP}$ ($10^3$ cm$^{-1}$) | 3.53 | 3.53 |
| $\gamma_{LP}$ ($10^3$ cm$^{-1}$) | 0.48 | 0.48 |
| $1/\gamma_{UP}$ (fs) | 1.5 | 1.5 |
| $1/\gamma_{LP}$ (fs) | 11 | 11 |

Table S2: Parameters for the early times 2DES simulation in the global approach.

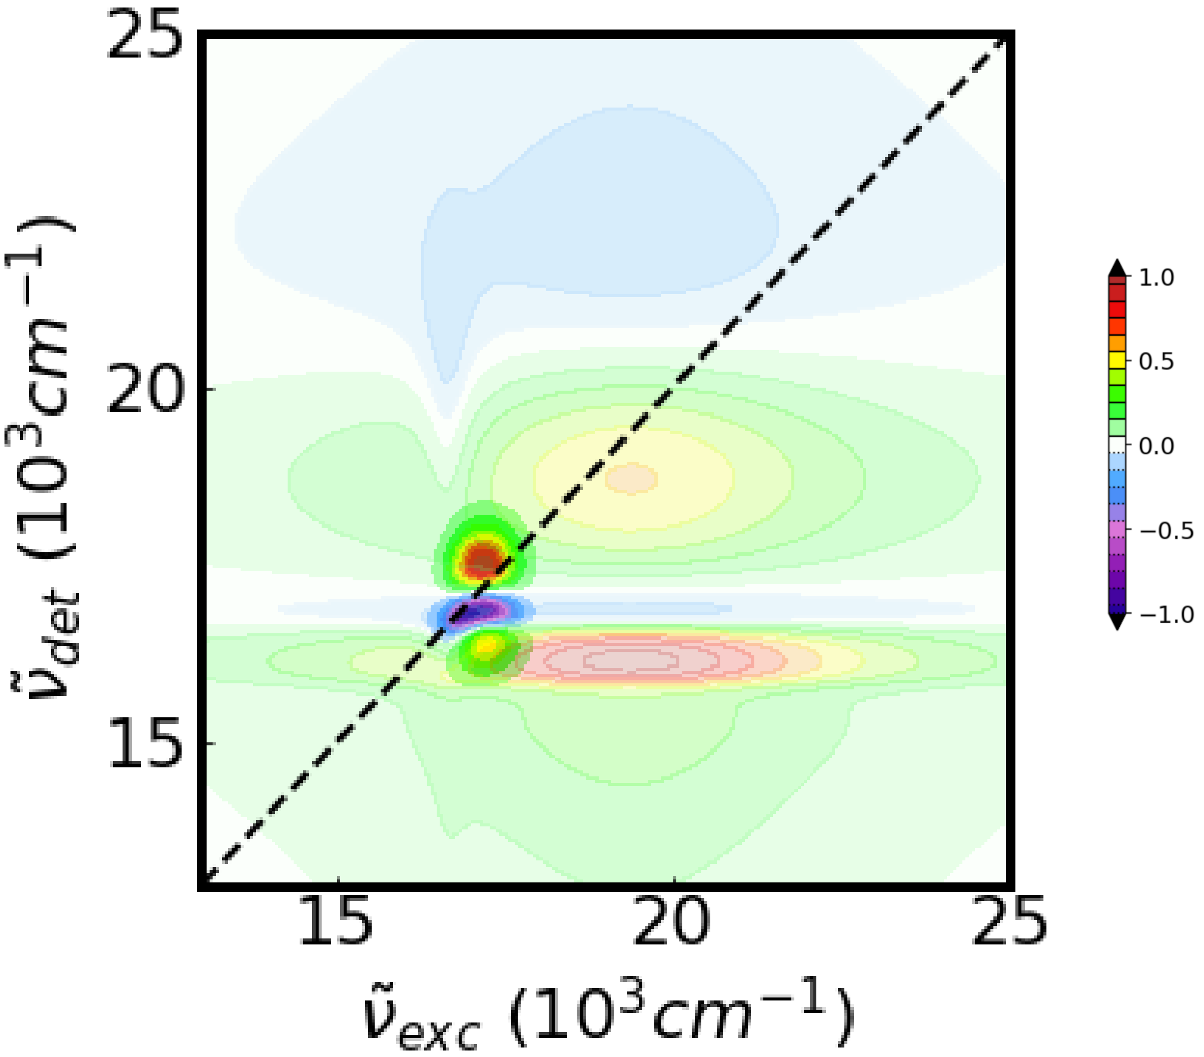


Figure S17: Early times simulations in the impulsive limit (semi-transparent) and with finite pulses (solid) for the local approach model.

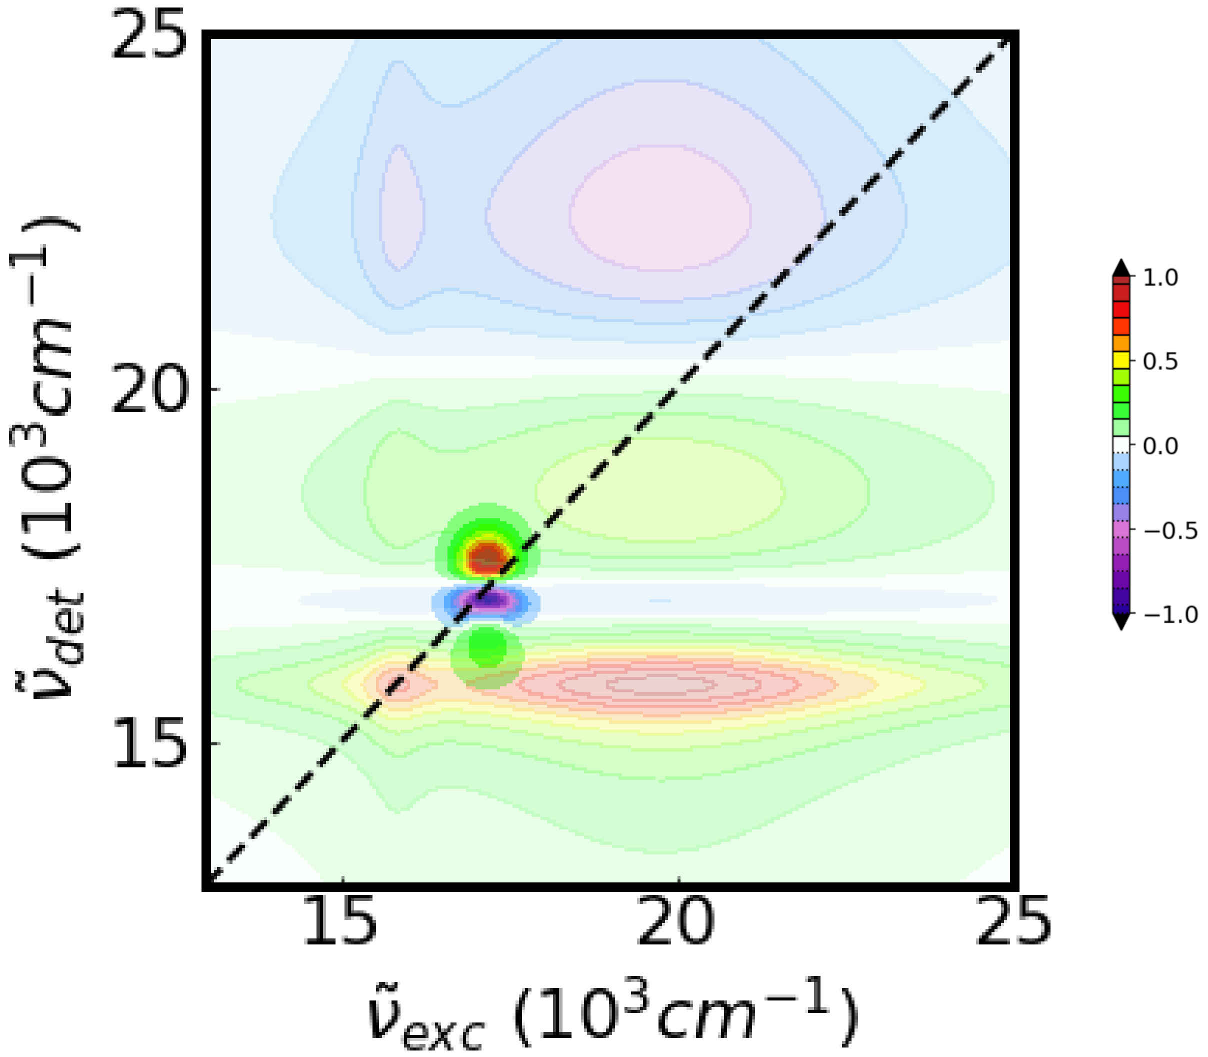


Figure S18: Early times simulations in the impulsive limit (semi-transparent) and with finite pulses (solid) for the global approach model.

## S5.2. Late times simulation

For the late time simulations we consider that the initial nonequilibrium distribution of electrons inside the metal has thermalized with the lattice, albeit at a temperature higher than room temperature. The thermal lattice expansion causes the conduction electron density to decrease which in turn decreases the plasma frequency ($\propto \sqrt{n/V}$, where $V$ is the unit cell volume and $n$ the number of conduction electrons per unit cell). While a pure redshift results in the general ordering of the negative and positive features observed, we have to allow for variations in the other parameters in order to reproduce the measured spectra quantitatively. Figures S19 (local approach) and S20 (global approach) show the simulations with a finite pulse (full fill) and in the impulsive limit (semi-transparent fill), respectively. As for the case of the early times, an unabmiguous fit of the spectra will require broadband experiments.

| Parameters | Ground state | Excited state |
|---|---|---|
| $\tilde{\nu}_{P1}$ ($10^3$ cm$^{-1}$) | 17.3 | 17.27 |
| $\tilde{\nu}_{J1}$ ($10^3$ cm$^{-1}$) | 16.73 | 16.75 |
| V ($10^3$ cm$^{-1}$) | 0.98 | 0.975 |
| $\mu_{p1}$ | 0.904 | 0.9 |
| $\mu_{j1}$ | 0.074 | 0.08 |
| $\gamma_{P1}$ ($10^3$ cm$^{-1}$) | 2.25 | 2.45 |
| $\gamma_{J1}$ ($10^3$ cm$^{-1}$) | 0.1701 | 0.151 |
| $1/\gamma_{P1}$ (fs) | 2.4 | 2.2 |
| $1/\gamma_{J1}$ (fs) | 31 | 35 |

Table S3: Parameters for the late times 2DES simulation in the local approach.

| Parameters | Ground state | Excited state |
|---|---|---|
| $\tilde{\nu}_{P1}$ ($10^3$ cm$^{-1}$) | 18.6 | 18.5 |
| $\tilde{\nu}_{J1}$ ($10^3$ cm$^{-1}$) | 16.75 | 16.77 |
| V ($10^3$ cm$^{-1}$) | 0.757 | 0.769 |
| $\mu_{p1}$ | 0.969 | 0.99 |
| $\mu_{j1}$ | 0.001 | 0.051 |
| $\gamma_{UP}$ ($10^3$ cm$^{-1}$) | 2.29 | 2.53 |
| $\gamma_{LP}$ ($10^3$ cm$^{-1}$) | 0.381 | 0.349 |
| $1/\gamma_{UP}$ (fs) | 2.3 | 2.1 |
| $1/\gamma_{LP}$ (fs) | 14 | 15 |

Table S4: Parameters for the late times 2DES simulation in the global approach.

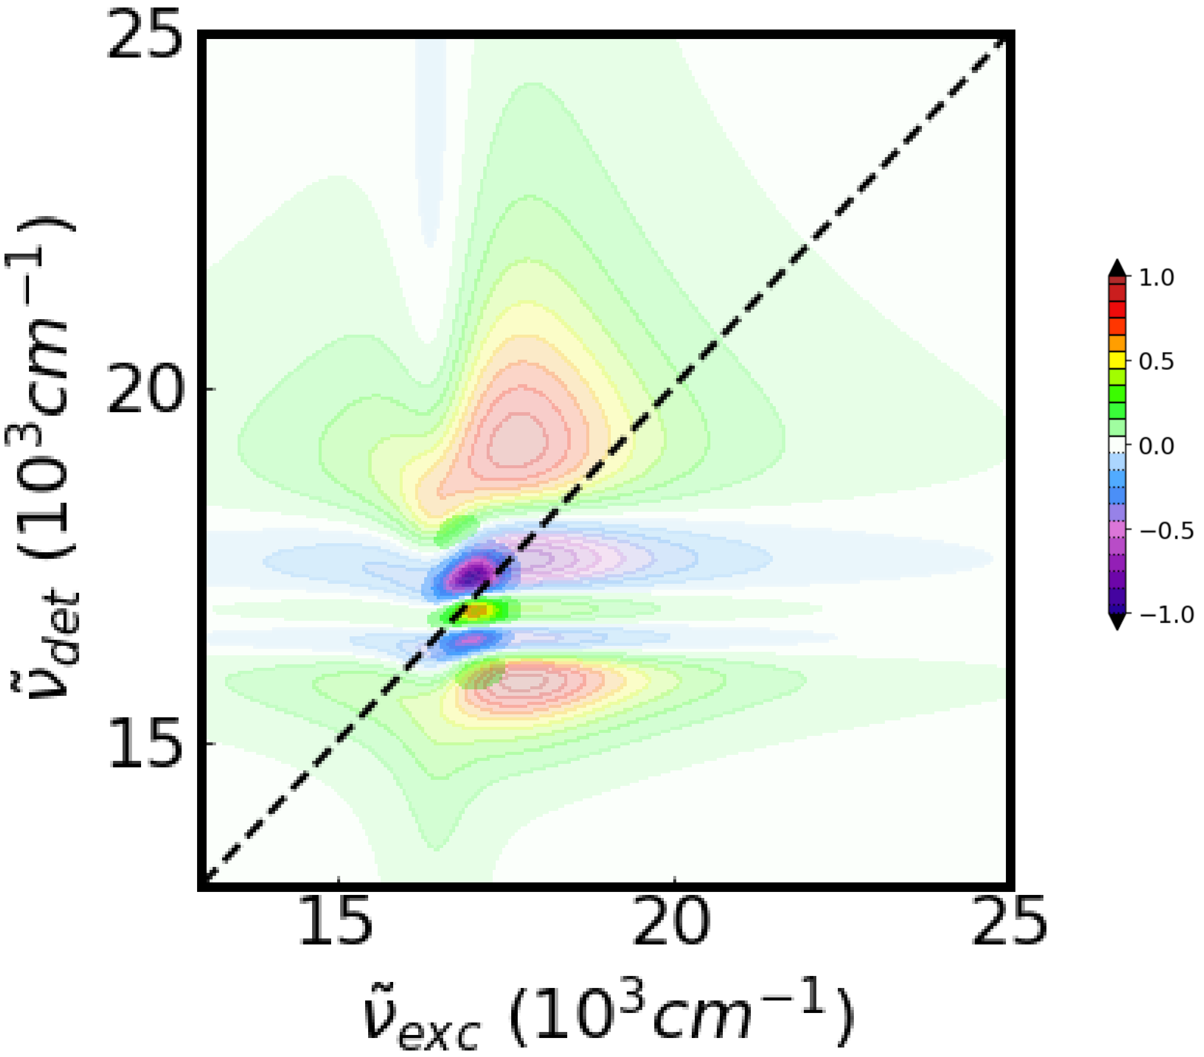


Figure S19: Late times simulations in the impulsive limit (semi-transparent) and with finite pulses (solid) for the local approach model.

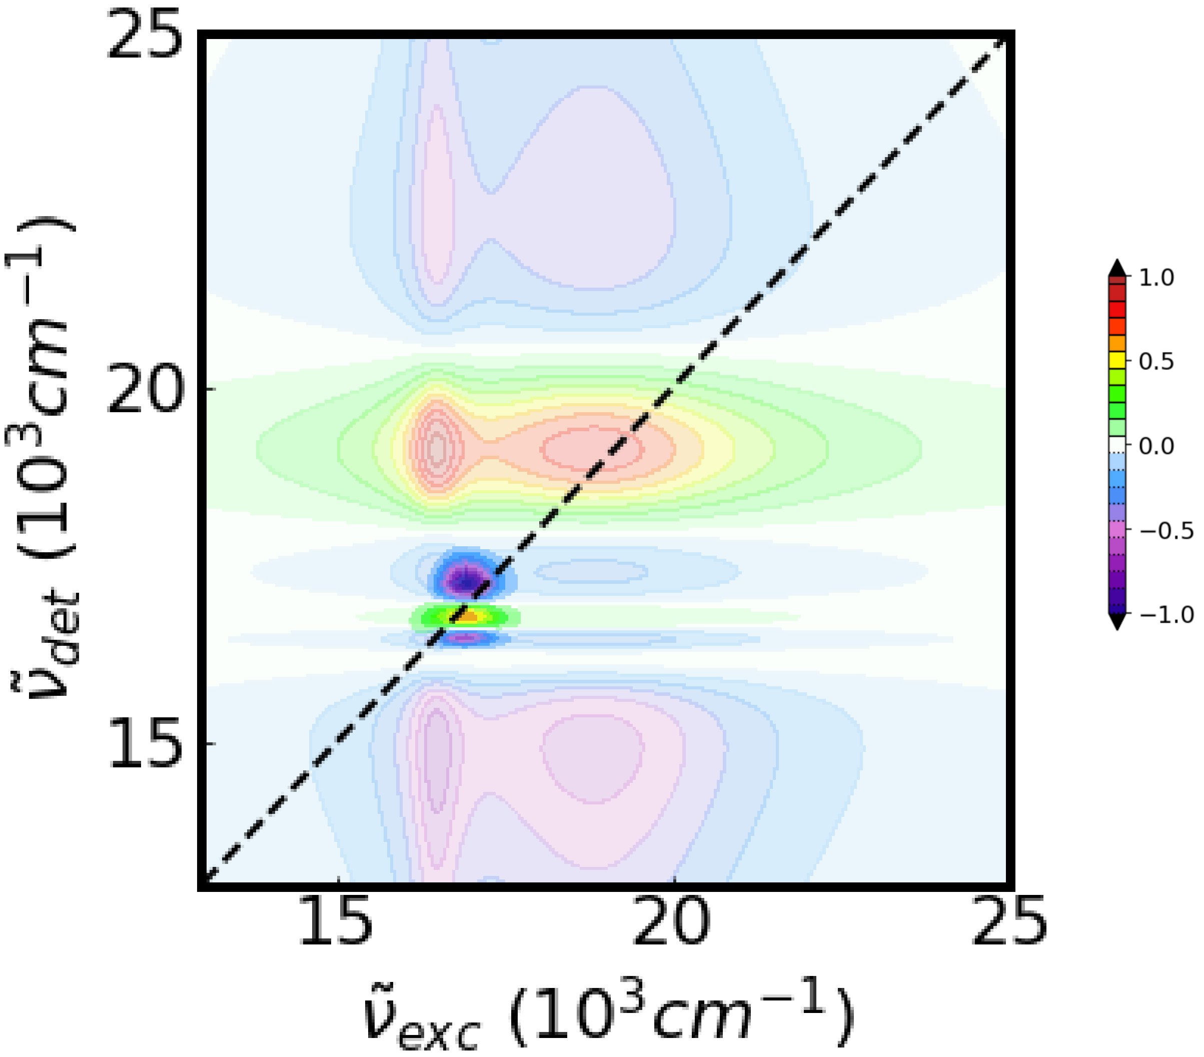


Figure S20: Late times simulations in the impulsive limit (semi-transparent) and with finite pulses (solid) for the global approach model.

# Note S6. Supplemental references

[1] Balci, S. (2013). Ultrastrong plasmon-exciton coupling in metal nanoprisms with J-aggregates. Opt. Lett. *38*, 4498–4501.

[2] Do, T. N., Gelin, M. F. and Tan, H.-S. (2017). Simplified expressions that incorporate finite pulse effects into coherent two-dimensional optical spectra. The Journal of Chemical Physics *147*, 144103.

[3] F. Ribeiro, R., Dunkelberger, A. D., Xiang, B., Xiong, W., Simpkins, B. S., Owrutsky, J. C. and Yuen-Zhou, J. (2018). Theory for Nonlinear Spectroscopy of Vibrational Polaritons. J. Phys. Chem. Lett. *9*, 3766–3771.

[4] Hofer, P. P., Perarnau-Llobet, M., Miranda, L. D. M., Haack, G., Silva, R., Brask, J. B. and Brunner, N. (2017). Markovian master equations for quantum thermal machines: local versus global approach. New Journal of Physics *19*, 123037.

[5] Link, S., Burda, C., Wang, Z. L. and El-Sayed, M. A. (1999). Electron dynamics in gold and goldsilver alloy nanoparticles: The influence of a nonequilibrium electron distribution and the size dependence of the electronphonon relaxation. The Journal of Chemical Physics *111*, 1255–1264.

[6] Molina, R. A., Weinmann, D. and Jalabert, R. A. (2002). Oscillatory size dependence of the surface plasmon linewidth in metallic nanoparticles. Phys. Rev. B *65*, 155427.

[7] Mukamel, S. (1995). Principles of nonlinear optical spectroscopy. Oxford University Press.

[8] Perner, M., Gresillon, S., März, J., von Plessen, G., Feldmann, J., Porstendorfer, J., Berg, K.-J. and Berg, G. (2000). Observation of Hot-Electron Pressure in the Vibration Dynamics of Metal Nanoparticles. Phys. Rev. Lett. *85*, 792–795.

[9] Sun, C.-K., Vallée, F., Acioli, L. H., Ippen, E. P. and Fujimoto, J. G. (1994). Femtosecond-tunable measurement of electron thermalization in gold. Phys. Rev. B *50*, 15337–15348.

[10] Voisin, C., Del Fatti, N., Christofilos, D. and Vallée, F. (2001). Ultrafast Electron Dynamics and Optical Nonlinearities in Metal Nanoparticles. The Journal of Physical Chemistry B *105*, 2264–2280.

[11] Voisin, C., Fatti, N. D., Christofilos, D. and Vallée, F. (2000). Time-resolved investigation of the vibrational dynamics of metal nanoparticles. Applied Surface Science *164*, 131 – 139.

[12] Weick, G., Molina, R. A., Weinmann, D. and Jalabert, R. A. (2005). Lifetime of the first and second collective excitations in metallic nanoparticles. Phys. Rev. B *72*, 115410.
